# Supplementary material for: ALIGNet: Partial-Shape Agnostic Alignment via Unsupervised Learning
Source: arXiv:1804.08497 source file (2018-10-30)
Supplement: Supplementary file 1 [file appendix.tex]

%\appendix
\begin{appendices}

\section{Optimization for Full Shapes}
\label{sec:optimization}

Given a particular non-partial source and target image, we would like to compute the optimal cage such that

\begin{equation}
\hat{W_c} = \min_{W_c} || S \oland W_c - T || = \min_{W_c} || \hat{T} - T ||
\end{equation}

However, optimizing such a cost function is non-trivial (and non-convex ?) due to the bilinear sampling operations. However, analogous to training Neural Networks (a highly complex and non-convex optimization problem) we can use the chain-rule to compute the gradient of this cost function.

\begin{equation}
\nabla_{W_c} = \frac{ \partial L^H(T,\hat{T})}{\partial \hat{W_c}} = 
\frac{ \partial L^H(T,\hat{T})}{\partial \hat{T}} \cdot 
\frac{\partial \hat{T}}{O_n }
\dots
\frac{O_1 }{\partial \hat{W_c}}
\end{equation}

Where $O_i \dots O_n$ are the operations which when applied to $W_c$ will result in the target image $T = O_n(O_1(W_c))$. This gradient along with an optimizer ({\em e.g.,} gradient descent or ADAM), will converge to a good solution.

\end{appendices}
